# Supplementary material for: BSD-GAN: Branched Generative Adversarial Network for Scale-Disentangled Representation Learning and Image Synthesis
Source: arXiv:1803.08467 source file (2020-08-04)
Supplement: Supplementary file 1 [file supp.tex]

\section{Appendix}
\subsection{Networks architecture and hyperparameters}

Code for the models is available will be made available. The detailed information about the networks architecture of generators and discriminators are presented in Table \ref{table:arc256-g}, \ref{table:arc256-d}, \ref{table:arc400-300-g}, \ref{table:arc400-300-d}. The non-architecture hyper-parameters are listed in Table \ref{table:hyper}. Please note that lrelu is leaky relu layer.

%https://github.com/duxingren14/BranchGAN

\noindent
\tabcolsep=0.11cm
\begin{table}
\begin{center}
\begin{tabular}{c||c|c}
\hline
    &  activation size &   filter  size   \\
		\hline
				\hline
input &   [30], [30],  &    NA   \\
& [30], [30], [30] &\\
\hline
concat &       [150]   &   NA  \\
linear &    [32768]             &     [32768,150]\\
reshape &    [8,8,512]       &  NA \\
deconv+instanceNorm+lrelu   &    [16,16,256]      &   [5,5,512,256]  \\
deconv+instanceNorm+lrelu   &    [32,32,128]      &   [5,5,256,128]  \\
deconv+instanceNorm+lrelu  &    [64,64,64]      &   [5,5,128,64]  \\
deconv+instanceNorm+lrelu   &    [128,128,64]      &   [5,5,64,64]  \\
deconv+sigmoid (output)   &    [256,256,3]      &   [5,5,64,3]  \\
\hline
\end{tabular}
\caption{Network architecture of the generator for $256 \times 256$ image synthesis.} \label{table:arc256-g}
\end{center}
\end{table}

\tabcolsep=0.11cm
\begin{table}
\begin{center}
\begin{tabular}{c||c|c}
\hline
    &  activation size &   filter  size   \\
		\hline
		\hline
input &   [256,256,3]  &    NA   \\
deconv+instanceNorm+lrelu   &    [128,128,64]     &   [5,5,3,64]  \\
deconv+instanceNorm+lrelu   &    [64,64,64]      &   [5,5,64,64]  \\
deconv+instanceNorm+lrelu  &    [32,32,128]      &   [5,5,64,128]  \\
deconv+instanceNorm+lrelu   &    [16,16,256]      &   [5,5,128,256]  \\
deconv+instanceNorm+lrelu   &    [8,8,512]      &   [5,5,256,512]  \\
reshape   &    [32768]      &   NA  \\
linear &      [1]    &    [32768,1]  \\
\hline
\end{tabular}
\caption{Network architecture of the discriminator for $256 \times 256$ image synthesis.} \label{table:arc256-d}
\end{center}
\end{table}
\noindent

\tabcolsep=0.11cm
\begin{table}
\begin{center}
\begin{tabular}{c||c|c}
\hline
    &  activation size &   filter  size   \\
		\hline
		\hline
input &   [30], [30], &    NA   \\
& [30], [30], [30] &\\
\hline
concat &       [150]   &   NA  \\
linear &    [17920]             &     [17920,150]\\
reshape &    [5,7,512]       &  NA \\
deconv+instanceNorm+lrelu   &    [10,13,256]      &   [5,5,512,256]  \\
deconv+instanceNorm+lrelu   &    [19,25,128]      &   [5,5,256,128]  \\
deconv+instanceNorm+lrelu  &    [37,50,64]      &   [5,5,128,64]  \\
deconv+instanceNorm+lrelu   &    [75,100,64]      &   [5,5,64,64]  \\
deconv+instanceNorm+lrelu  &    [150,200,64]      &   [5,5,64,64]  \\
deconv+sigmoid (output)   &    [300,400,3]      &   [5,5,64,3]  \\
\hline
\end{tabular}
\caption{Network architecture of the generator for $400 \times 300$ image synthesis.} \label{table:arc400-300-g}
\end{center}
\end{table}

\noindent
\tabcolsep=0.11cm
\begin{table}[!t]
\begin{center}
\begin{tabular}{c||c|c}
\hline
    &  activation size &   filter  size   \\
		\hline
		\hline
input &   [300,400,3]  &    NA   \\
deconv+instanceNorm+lrelu   &    [150,200,64]     &   [5,5,3,64]  \\
deconv+instanceNorm+lrelu   &    [75,100,64]      &   [5,5,64,64]  \\
deconv+instanceNorm+lrelu  &    [38,50,64]      &   [5,5,64,64]  \\
deconv+instanceNorm+lrelu   &    [19,25,128]      &   [5,5,64,128]  \\
deconv+instanceNorm+lrelu   &    [10,13,256]      &   [5,5,128,256]  \\
deconv+instanceNorm+lrelu   &    [5,7,512]      &   [5,5,256,512]  \\
deconv+instanceNorm+lrelu   &    [17920]      &   NA \\
linear &      [1]    &    [17920,1]  \\
\hline
\end{tabular}
\caption{Network architecture of the discriminator for $400 \times 300$ image synthesis.} \label{table:arc400-300-d}
\end{center}
\end{table}

\tabcolsep=0.11cm
\begin{table}[!t]
\begin{center}
\begin{tabular}{c||c}
\hline
name &  value   \\
		\hline
		\hline
Optimizer&  AdamOptimizer       \\
learning rate &  0.0002   \\
beta1 &       0.5         \\
beta2 &    0.999       \\
		\hline
\#sub-vector   &  5 for 256 $\times$ 256 images      \\
 &   6 for 512 $\times$ 512 or 400 $\times$ 300 images        \\
		\hline
\#epoch/scale   &   20 for 256 $\times$ 256 images       \\
  &   12 for 512 $\times$ 512 or 400 $\times$ 300 images     \\
			\hline
\#batch/epoch  &   subject to dataset size and batch size    \\
  &   we use full dataset for each epoch \\
			\hline
batch size &   20 for 256 $\times$ 256 images    \\
&  12 for 512 $\times$ 512 or 400 $\times$ 300 images     \\
\hline
\end{tabular}
\caption{Non-architecture training hyperparameters.} \label{table:hyper}
\end{center}
\end{table}
\noindent

\subsection{Initialization of neural weights, ``freeze'' and ``defreeze''}

For the untrained linear or deconv/conv/linear layers, the filter weights are initialized with normally random numbers $N(\mu,\sigma)$ and biases are initialized with $0$. For instance normalization layer, we initialize the $scale$ with 1.0 and assign the $center$ with 0.0. 

We ``freeze'' certain branches (or weights) by feeding the corresponding $\mathbf{z}$ vector with $\mathbf{0}$. Here we intend to explain the reason why feeding zero vector makes the corresponding weights untrainable.

 Therefore, the activations of linear layer when fed with $\mathbf{0}$ are given by $f(\mathbf{0}) \equiv  \mathbf{\theta}\mathbf{0}+\mathbf{0}  \equiv \mathbf{0}$, where $\mathbf{\theta}$ are the linear weights. The activations of conv/deconv layer are given by $f(\mathbf{0})  \equiv \mathbf{\theta}  \circledast  \mathbf{0} + \mathbf{0}  \equiv \mathbf{0}$ (or $\mathbf{\theta}  \circledast  \mathbf{0} \equiv \mathbf{0}$ after concatenation), where $\mathbf{\theta}$ are filter weights. So we have the gradients $\nabla f_\mathbf{\theta}(\mathbf{0}) \equiv \mathbf{0}$. For instance normalization layer and leaky relu layer, $g(\mathbf{0})  \equiv lrelu((\mathbf{0}-\mathbf{0})  \cdot  \mathbf{1.0} + \mathbf{0.0})  \equiv \mathbf{0}$. We have the gradients $g_\mathbf{\beta}(\mathbf{0}) \equiv \mathbf{0}$, where $\beta$ is the scale.

In this way, the branches (or weights) could be ``frozen'' when fed with $\mathbf{0}$.
To ``defreeze'' these branches (or weights), simply feed them with non-zero vectors.

\subsection{Branch suppression}
\label{subsec:supp}
We observed ``branch suppression'' in all kinds of multi-branch generators as shown in Figure~\ref{fig:ps}, among which some are fully suppressed, some are partially suppressed. In ``branch suppression'', the already-trained weights (branches) will have priority in maintaining their role in encoding the image structures that are already well encoded and suppress the other branches. To explain it in more details, we present a few examples of branch suppression in Figure~\ref{fig:ps}.
\noindent
\begin{figure*}[!t]
\begin{center}
\includegraphics[width=\linewidth]{figures/ps2}

\includegraphics[width=\linewidth]{figures/ps3}
\caption{Two examples of branch suppression in GANs. In these examples, we employ the training loss and discriminator of dcgan~\cite{radford2015unsupervised}. Here we change the architecture of the generator a bit by conditioning image generation on split $\mathbf{z}$ vectors ($\mathbf{z}^t, t \in \{1,2,3\}$). 
In the upper row, the left branch is already well trained for image generation, and the middle and right branches are initialized randomly (see more details about the initialization in the supplementary material). Then we train the GAN by following the standard GAN training procedure as in~\cite{radford2015unsupervised}. After the training converges, the left branch dominates the output while the other are fully suppressed, as seen from the variance image on the right (see Fig. \ref{fig:face256-1} for the meaning of variance image). In the lower row, the generator architecture is the same as traditional GAN except that the $\mathbf{z}$ vector is split. We train the left branch till converging, then de-freeze the middle branch for training till converging, and finally the right branch. Note that the number of training steps for each stage are equal and the pre-trained weights (or branches) are not frozen even after new branches are de-frozen. As a result, the middle branch is slightly suppressed and the right branch is severely suppressed as seen from the rightmost variance images.} \label{fig:ps}
\end{center}
\end{figure*}

\subsection{More image editing results with BranchGAN and iGAN}
Figure \ref{fig:face512-branch} shows the outputs of BranchGAN on $celeba\_hq$ 512 $\times$ 512 dataset.

Figures \ref{fig:fusion4} shows more results of cross-scale image fusion. 

Figures \ref{fig:face256}, \ref{fig:face512}, \ref{fig:igan-face256}, \ref{fig:car-igan} and \ref{fig:lsun-igan} show more results of iGAN using our multi-scale image manifold as the latent codes.

%\begin{figure*}[!t]
%\begin{center}
%\includegraphics[width=0.8\linewidth]{figures/fusion_examples/0_0}
%\includegraphics[width=0.8\linewidth]{figures/fusion_examples/0_1}
%\includegraphics[width=0.8\linewidth]{figures/fusion_examples/0_2}
%\includegraphics[width=0.8\linewidth]{figures/fusion_examples/0_3}
%\includegraphics[width=0.8\linewidth]{figures/fusion_examples/0_4}
%\includegraphics[width=0.8\linewidth]{figures/fusion_examples/0_5}
%\caption{Results of {\em Cross-scale image fusion.\/} The notations and synthesis setup are the same as in Figure~\ref{fig:fusion}.}
%\label{fig:fusion2}
%\vspace{-25pt}
%\end{center}
%\end{figure*}
%
%\begin{figure*}[!t]
%\begin{center}
%\includegraphics[width=0.8\linewidth]{figures/fusion_examples/1_0}
%\includegraphics[width=0.8\linewidth]{figures/fusion_examples/1_1}
%\includegraphics[width=0.8\linewidth]{figures/fusion_examples/1_2}
%\includegraphics[width=0.8\linewidth]{figures/fusion_examples/1_3}
%\includegraphics[width=0.8\linewidth]{figures/fusion_examples/1_4}
%\includegraphics[width=0.8\linewidth]{figures/fusion_examples/1_5}
%\caption{Results of {\em Cross-scale image fusion.\/} The notations and synthesis setup are the same as in Figure~\ref{fig:fusion}.}
%\label{fig:fusion3}
%\vspace{-25pt}
%\end{center}
%\end{figure*}

\begin{figure*}[!t]
\begin{center}
\includegraphics[width=0.8\linewidth]{figures/fusion_examples/2_0}
\includegraphics[width=0.8\linewidth]{figures/fusion_examples/2_1}
\includegraphics[width=0.8\linewidth]{figures/fusion_examples/2_2}
\includegraphics[width=0.8\linewidth]{figures/fusion_examples/2_3}
\includegraphics[width=0.8\linewidth]{figures/fusion_examples/2_4}
\includegraphics[width=0.8\linewidth]{figures/fusion_examples/2_5}
\caption{Results of {\em Cross-scale image fusion.\/} The notations and synthesis setup are the same as in Figure~\ref{fig:fusion}.}
\label{fig:fusion4}
\vspace{-25pt}
\end{center}
\end{figure*}
%
%\begin{figure*}[!t]
%\begin{center}
%\includegraphics[width=0.8\linewidth]{figures/fusion_examples/3_0}
%\includegraphics[width=0.8\linewidth]{figures/fusion_examples/3_1}
%\includegraphics[width=0.8\linewidth]{figures/fusion_examples/3_2}
%\includegraphics[width=0.8\linewidth]{figures/fusion_examples/3_3}
%\includegraphics[width=0.8\linewidth]{figures/fusion_examples/3_4}
%\includegraphics[width=0.8\linewidth]{figures/fusion_examples/3_5}
%\caption{Results of {\em Cross-scale image fusion.\/} The notations and synthesis setup are the same as in Figure~\ref{fig:fusion}.}
%\label{fig:fusion5}
%\vspace{-25pt}
%\end{center}
%\end{figure*}
%
%
%\begin{figure*}[!t]
%\begin{center}
%\includegraphics[width=0.8\linewidth]{figures/fusion_examples/0_6}
%\includegraphics[width=0.8\linewidth]{figures/fusion_examples/0_7}
%\includegraphics[width=0.8\linewidth]{figures/fusion_examples/1_6}
%\includegraphics[width=0.8\linewidth]{figures/fusion_examples/1_7}
%\includegraphics[width=0.8\linewidth]{figures/fusion_examples/2_6}
%\includegraphics[width=0.8\linewidth]{figures/fusion_examples/2_7}
%\caption{Results of {\em Cross-scale image fusion.\/} The notations and synthesis setup are the same as in Figure~\ref{fig:fusion}.}
%\label{fig:fusion6}
%\vspace{-25pt}
%\end{center}
%\end{figure*}

\noindent
\begin{figure*}[!t]
\begin{center}
\includegraphics[width=0.8\linewidth]{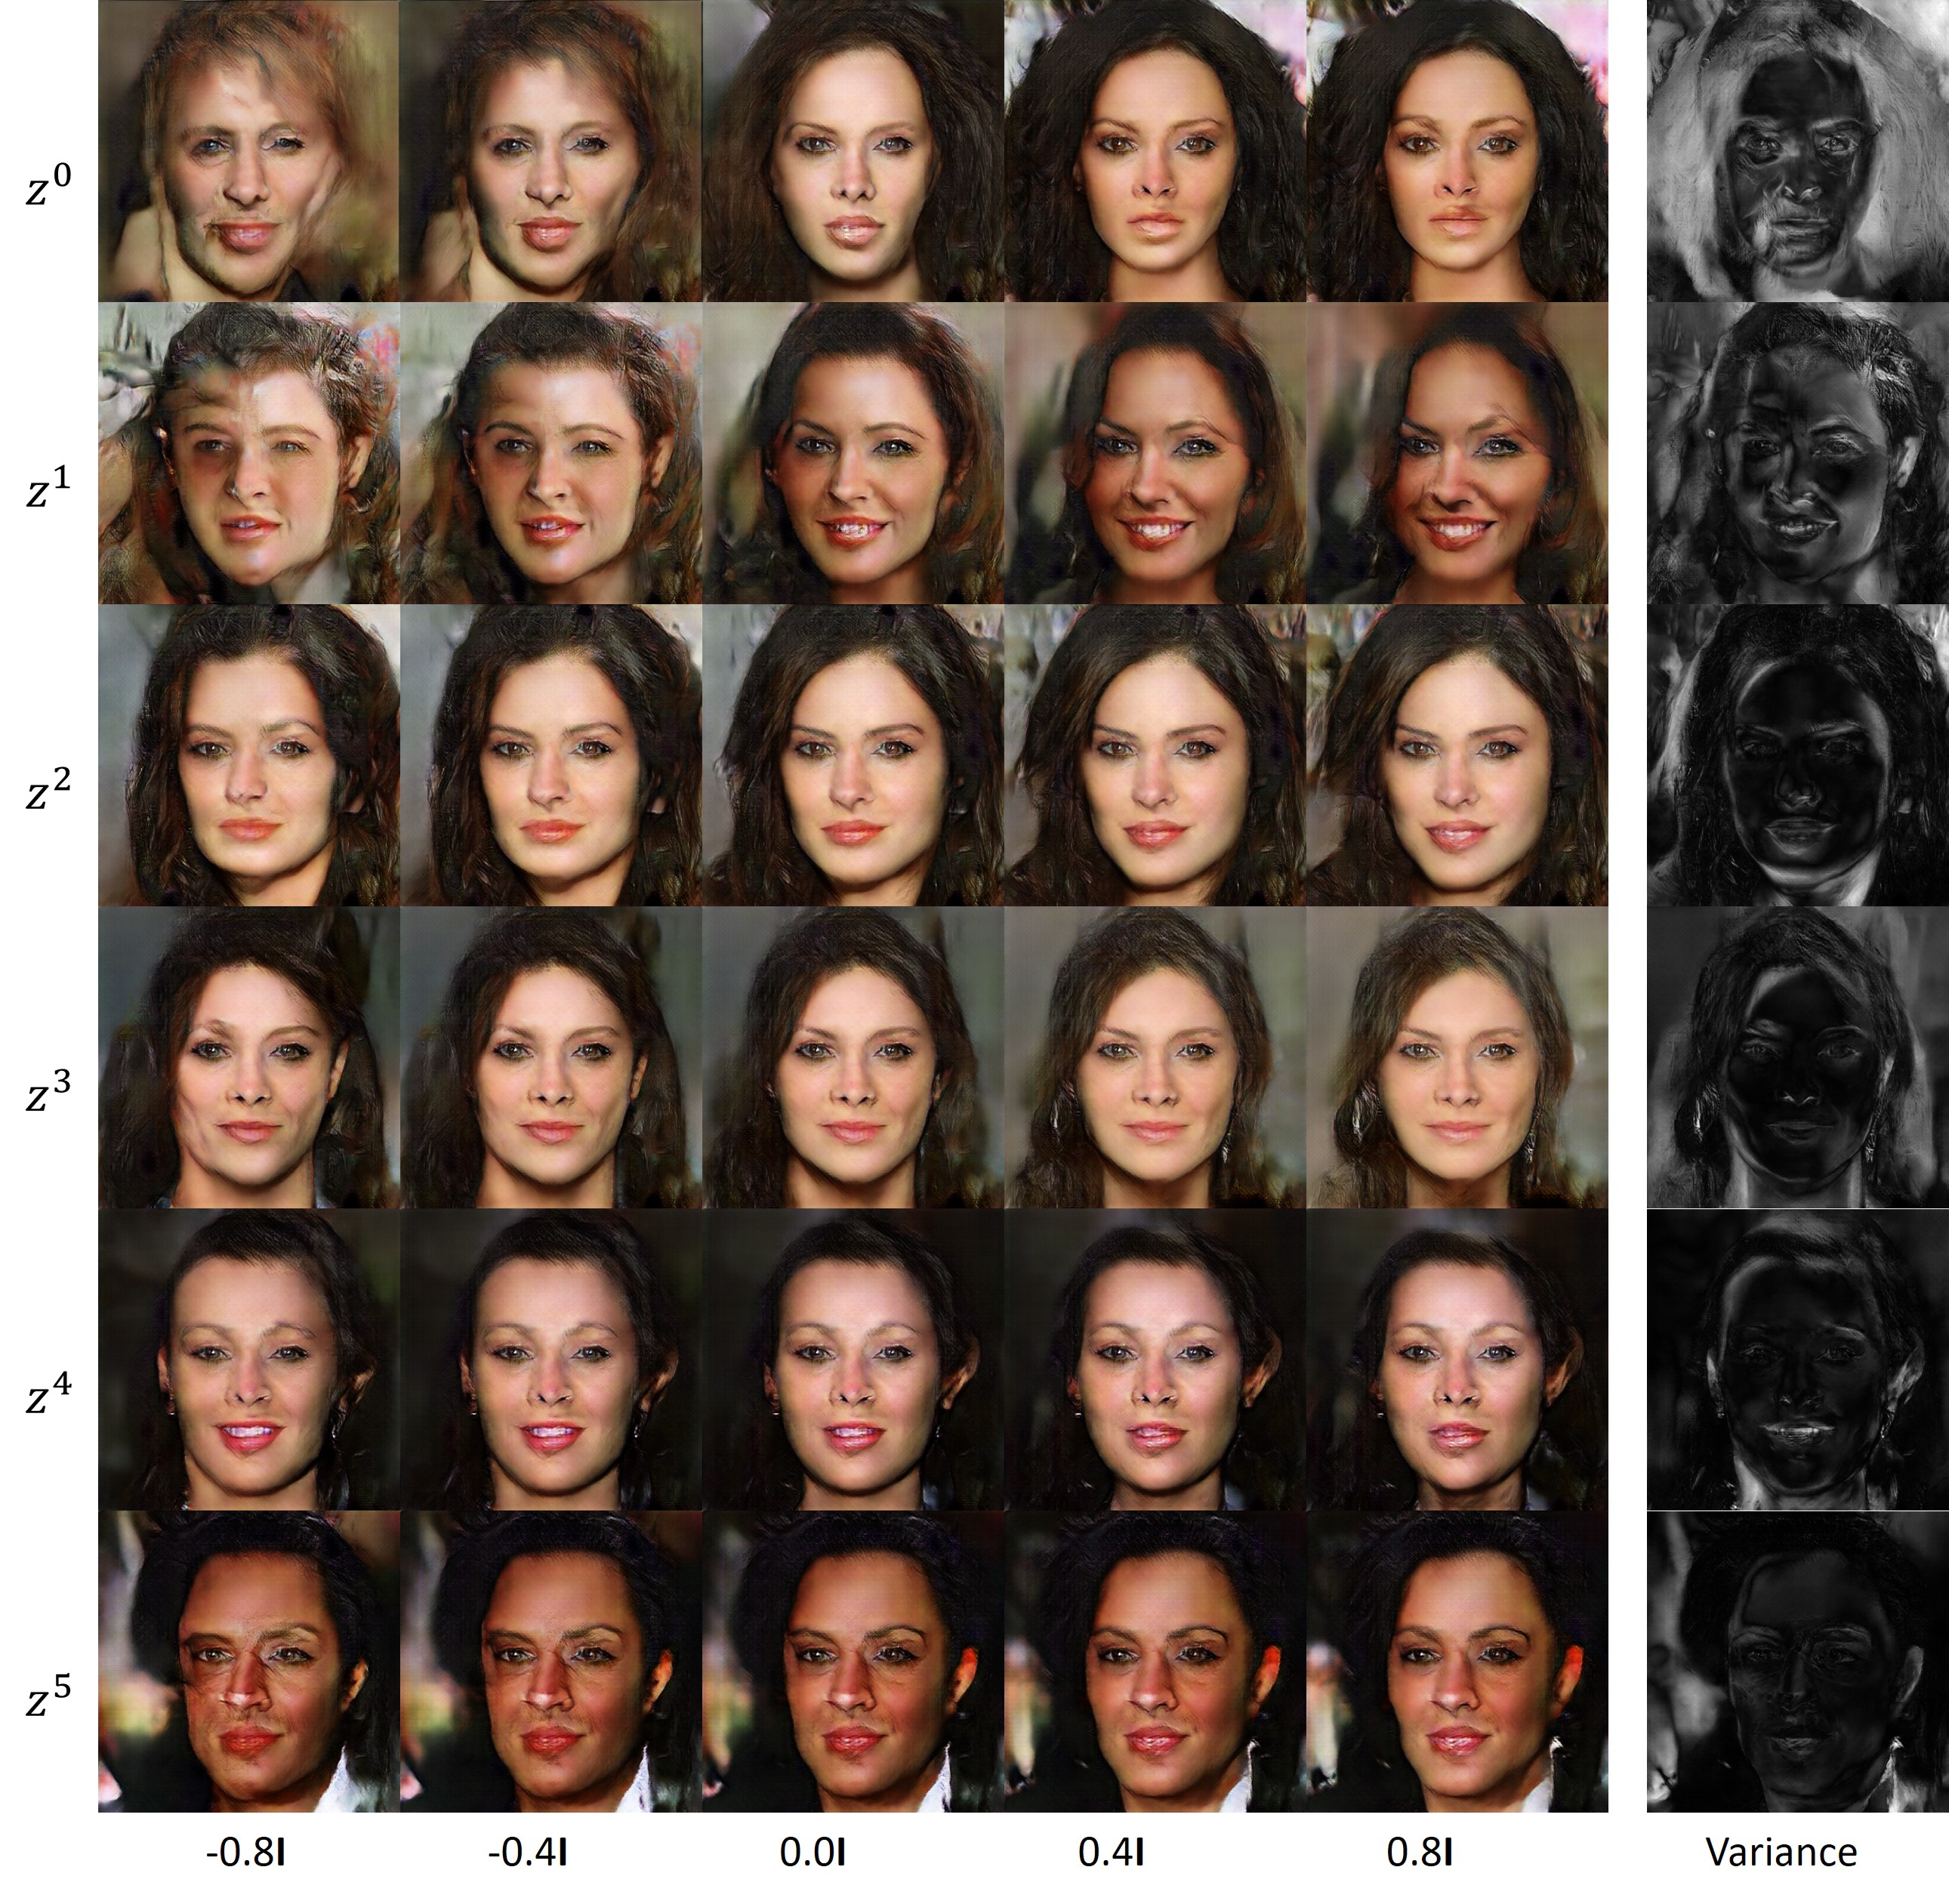}
\caption{{\em Effects on generated images for $celeba\_hq$ 512 $\times$ 512 dataset by varying individual sub-vectors.\/} The output setting is similar as in Figure~\ref{fig:face256-1} except that there is one more sub-vector $\mathbf{z}^5$ and each row is generated independently. From top to bottom, changing ${\mathbf{z}^t}$ ($t \in \{0, 1, 2, 3, 4, 5\}$) leads to smaller and smaller image variations, as reflected by intensity drop in the variance images. Similar to Figure~\ref{fig:face256-1}, sub-vector ${\mathbf{z}^0}$ dominates the overall color, ${\mathbf{z}^1}$ controls some facial features and hair features, while the rest bring minor changes near ear, mouth, and hair.} \label{fig:face512-branch}
\end{center}
\end{figure*}
\noindent

\noindent
\begin{figure*}[!t]
\begin{center}
\includegraphics[width=0.95\linewidth]{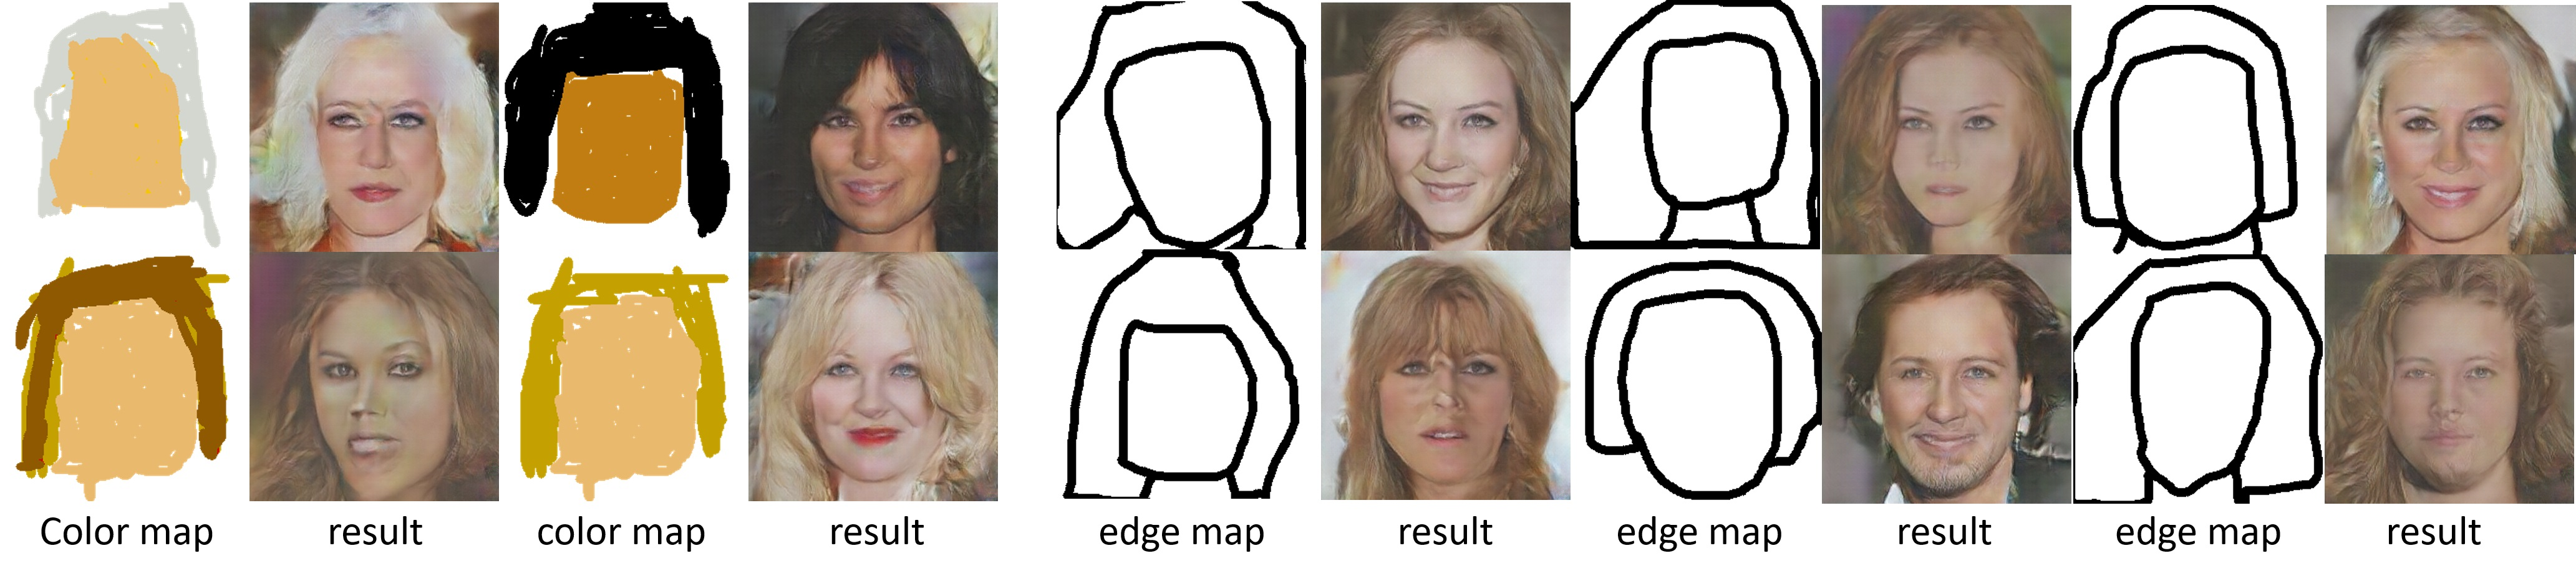}
\caption{The edge maps and color maps drawn by users and the corresponding image generation results with improved iGAN.} \label{fig:face256}
\end{center}
\end{figure*}

\begin{figure*}[!t]
\begin{center}
\includegraphics[width=\linewidth]{figures/edit-face-obsolete}
\caption{Edits by users and the corresponding results generated by improved iGAN. (a) face erased. (b) face slimmed. (c) mouth replaced with a patch from another image. (d) hair darkened. (e) mouth closed. (f) hair turned brown. (g) hair turned brown, eye shadowed, and lips reddened. (h) face whitened  and lips reddened.} \label{fig:igan-face256}
\end{center}
\end{figure*}

\begin{figure*}[!t]
\begin{center}
\includegraphics[width=\linewidth]{figures/512}
\caption{Face image (512x512) generation and editing results with improved iGAN. (a)-(b), results based on edge maps. (c)-(d), results based on masked color maps. (e)-(h), image editing results.} \label{fig:face512}
\end{center}
\end{figure*}

\begin{figure*}[!t]
\begin{center}
\includegraphics[width=\linewidth]{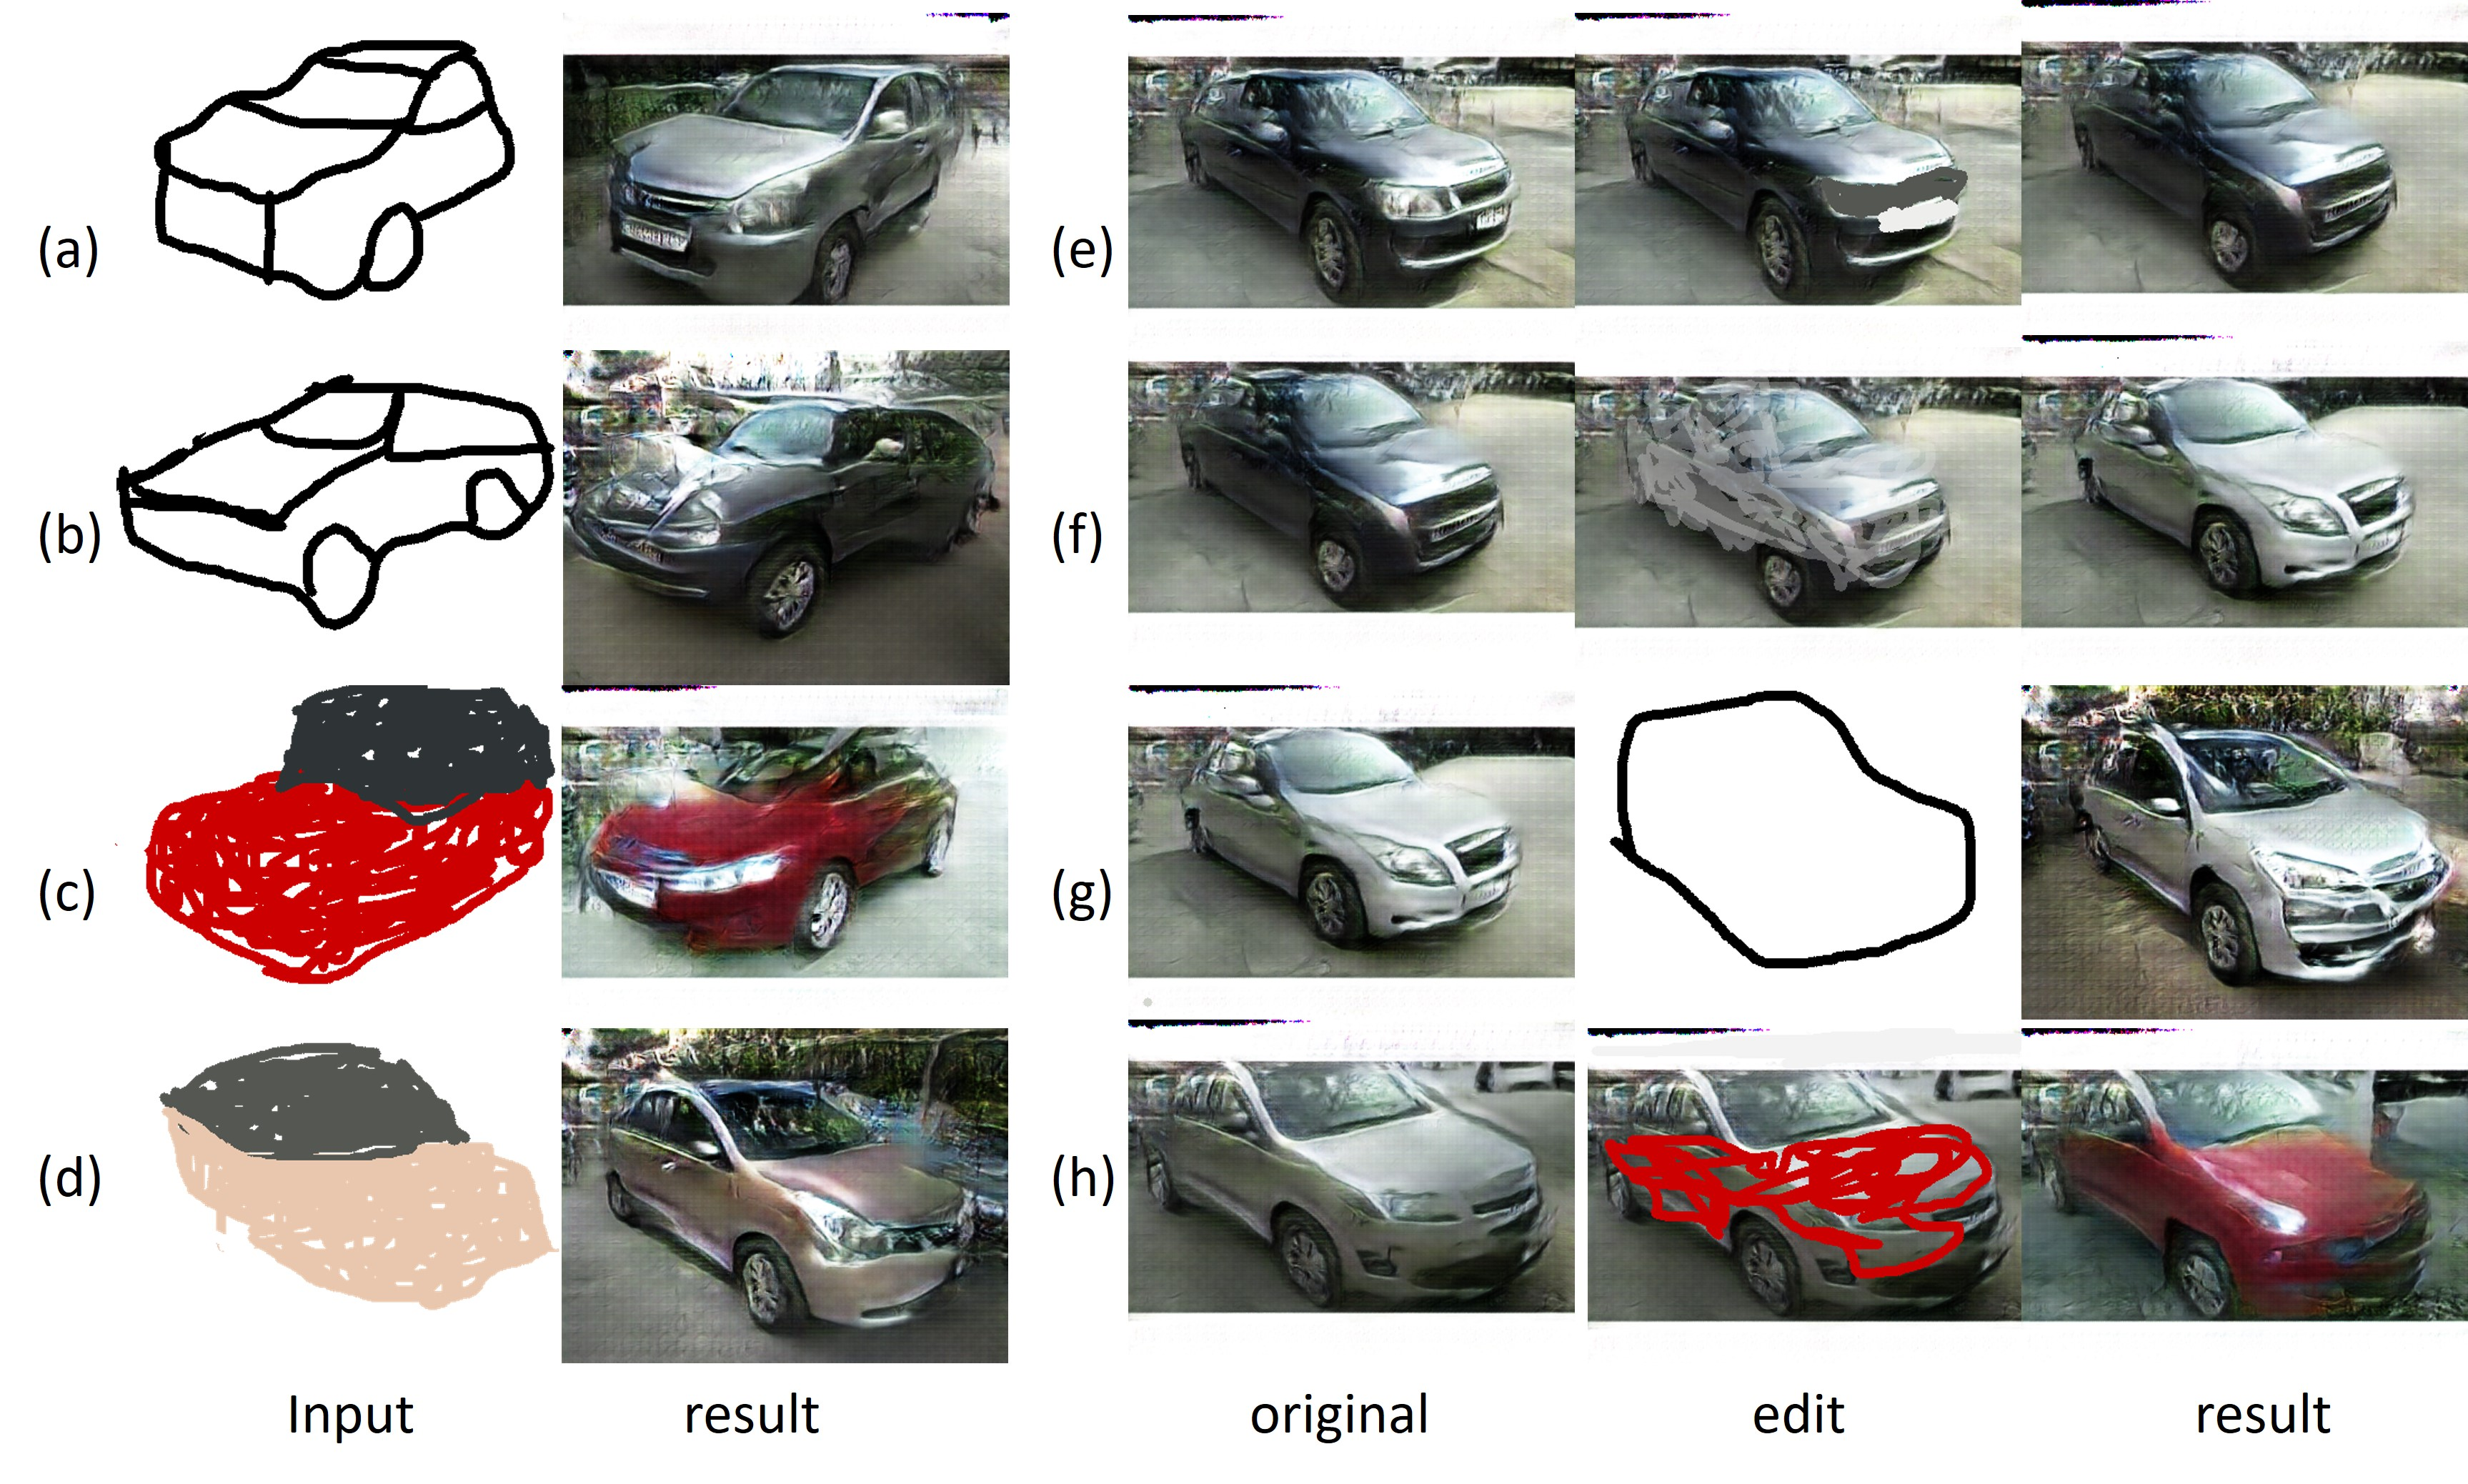}
\caption{Car image generation and editing results with improved iGAN: (a-b) results based on edge maps; (c-d) results based on masked color maps; (e-h) manipulation of existing images, including erasing license plate (e), changing body color (f \& h), and adding extra edge map (g).}
\label{fig:car-igan}
\end{center}
\end{figure*}

\begin{figure*}[!t]
\begin{center}
\includegraphics[width=\linewidth]{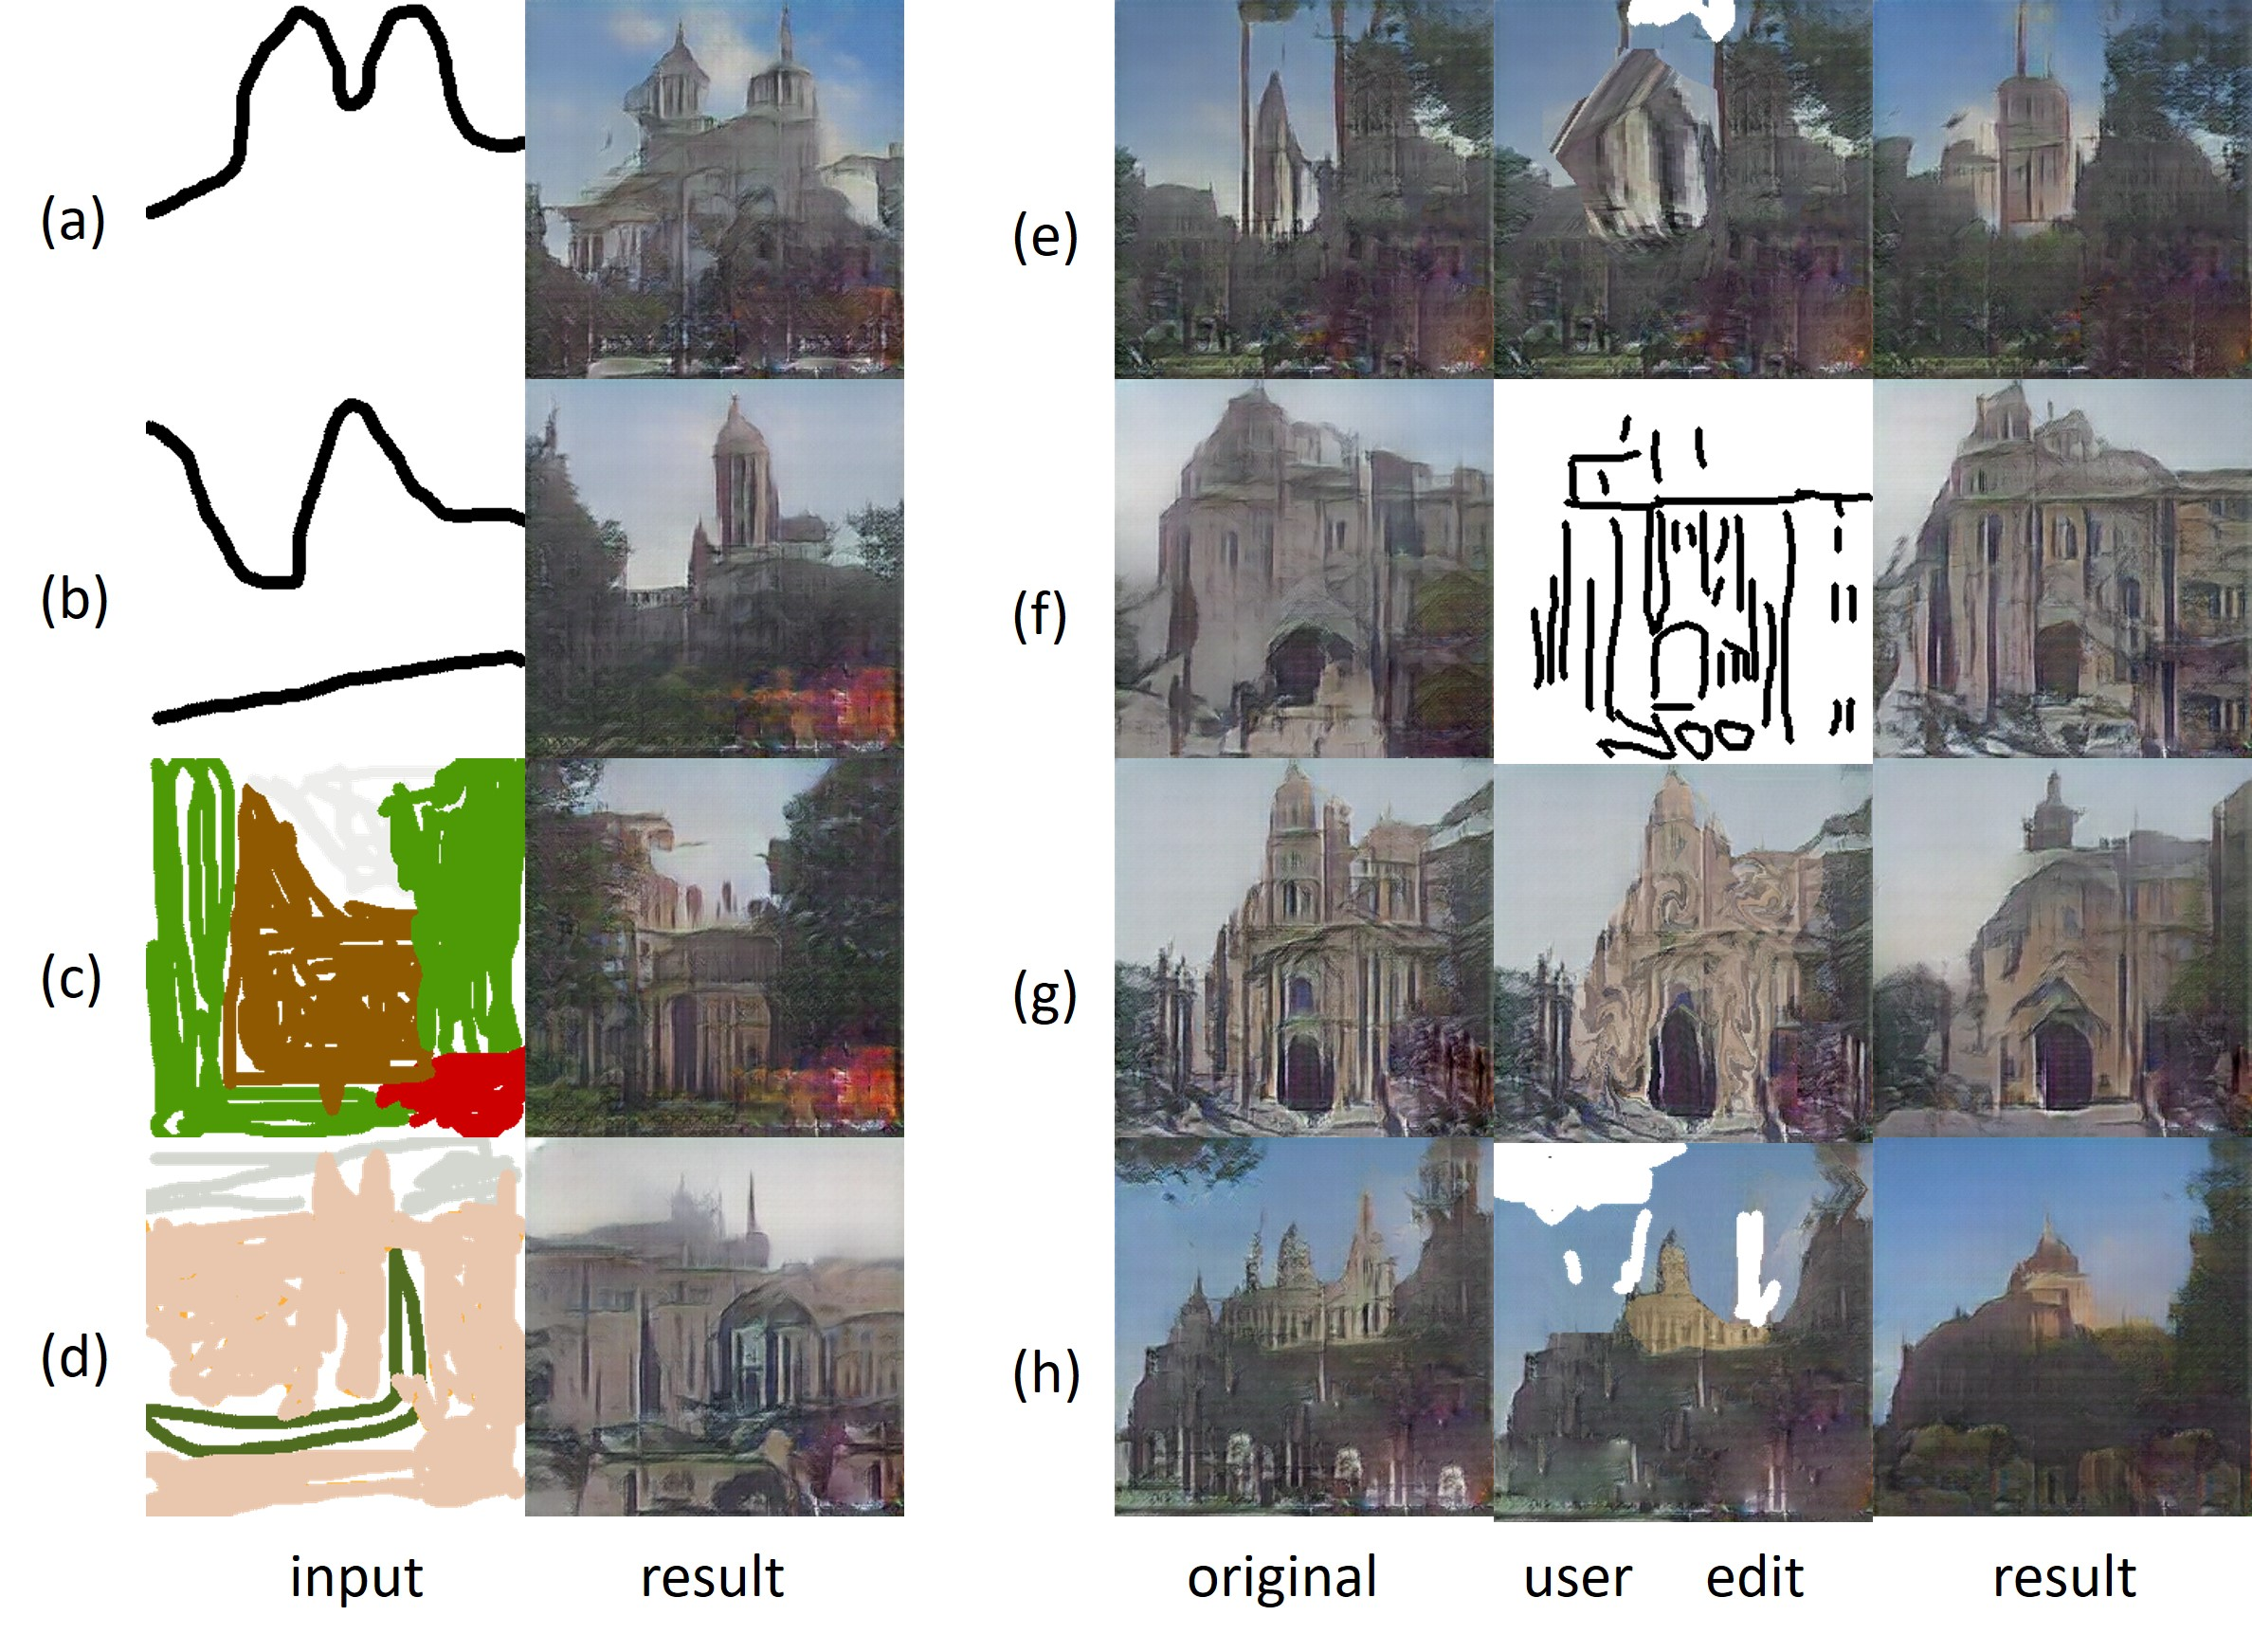}
\caption{Church image generation and editing results with improved iGAN: (a-b) results based on edge maps; (c-d) results based on masked color maps; and (e-h) image editing results.} \label{fig:lsun-igan}
\end{center}
\end{figure*}

\subsection{Consistency of $VBS$ with human perception}

We are not aware of universally accepted metrics to assess variation of outputs ``by scale", as Frechet Inception Distance and Inception Score do not. We proposed VBS as objective metrics for variation-by-scale. To assess consistency of the metric with human perception, we conducted a user study. We selected 48 pairs of result images (18 for each dataset) that were produced by controlling the value of different latent vectors of BranchGAN. We hired 20 Turkers to rate each pair in terms of level of variation. In the test, three options with elaborate explanations were shown to the Turkers: (a) large-scale variation; (b) median-scale variation; or (c) small-scale variation. The label with the most votes is treated as ground-truth. Then we compare the human-labeled results with those estimated by VBS (the scale level with highest score is used) and compute the percentages of agreements is 85,4\%. The agreement rates of VBS and human perception are quite high from this preliminary study (significantly better than random), serving as an initial validation. Further explorations are certainly warranted.

\subsection{Experiments with LAPGAN \cite{denton2015deep}}

LAPGAN \cite{denton2015deep} is very similar to BranchGAN in terms of coarse-to-fine image synthesis and adding noise at multiple scale level, though the noise is added though dropout layer, which is neither controllable nor explicit. We did re-implement LAPGAN and attempt to add noise vectors explicitly as inputs to generators at each step. The results showed that the noise vectors are not responsible for any variation of the residual images. The reason could be that by using strictly paired training data, the upscaled conditioning image would deterministically generate the residual image.
